# Supplementary material for: Deep Semi-Supervised Embedded Clustering (DSEC) for Stratification of Heart Failure Patients
Source: arXiv:2012.13233 source file (2021-01-17)
Supplement: Supplementary file 1 [file Supplementary_Material.pdf]

# Supplementary Material: Deep Semi-Supervised Embedded Clustering (DSEC) for Stratification of Heart Failure Patients

**Oliver Carr**[1] **Stojan Jovanovic**[1] **Luca Albergante**[1] **Fernando Andreotti**[1] **Robert Dürichen**[1] **Nadia Lipunova**[1] **Janie Baxter**[1] **Rabia Khan**[1] **Benjamin Irving**[1]

## 1. Deep Semi-Supervised Embedded Clustering (DSEC) Network

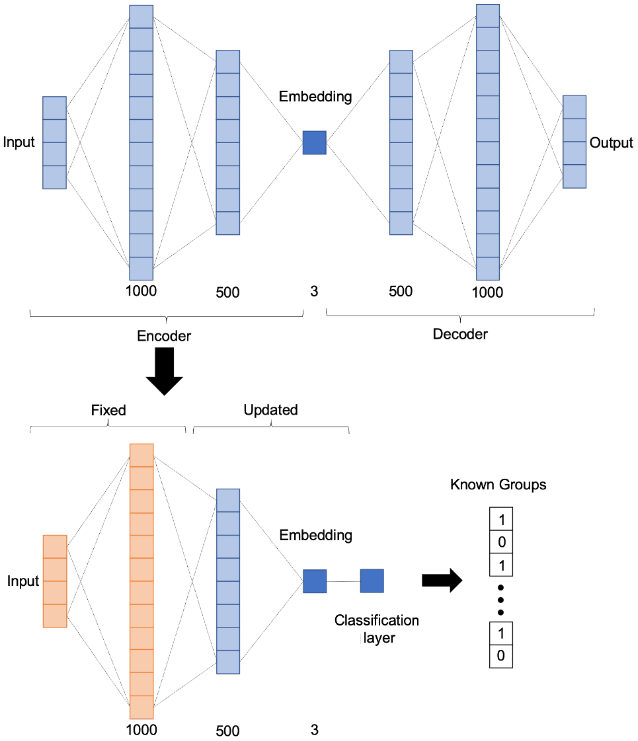


*Figure 1.* A schematic of the architecture used for DSEC and the steps performed when training using the autoencoder and classification losses.

Figure 1 shows the architecture used for the encoder and decoder of the deep semi-supervised embedded clustering (DSEC) model. The first and second layers having 1,000 and 500 hidden nodes respectively, with the embedding layer having 3 dimensions.

The diagram also shows how the network is updated through training on a classification problem. After removing the decoding layers, a classification layer is added after the embedding layer, all model weight are fixed except the penultimate two layers and these weights are updated using a binary cross entropy loss function.

Finally, the classification layer is removed and all layers of the encoder are updated using the Kullback Leibler divergence to separate clusters within the embedded space.

## 2. Embedded Space and Classification

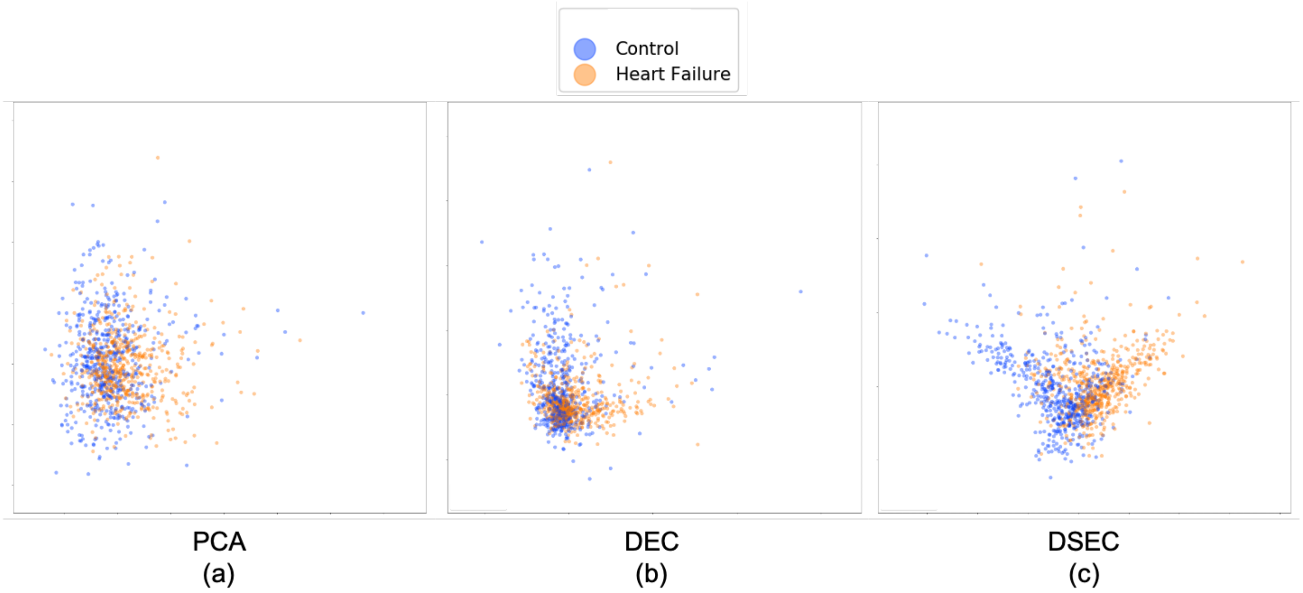


*Figure 2.* Scatter plots of the first two principal components of the embedded space found using principal component analysis (a), deep embedded clustering (DEC) (b), and DSEC (c). Each point represents a patient from the test set, with colours indicating whether the patient is from the heart failure or control cohort.

Figure 2 shows the first two principal components of the embedded space for each of the three models used to embed the patient data. Figure 2 (a) shows the embedding found using principal component analysis (PCA) and Figure 2 (b) shows the embedding found using deep embedded clustering (DEC). Both these methods of embedding show little separation between the heat failure and control patients. This is not unexpected due to being completely unsupervised methods. Figure 2 (c) show the embedded space found using DSEC, the heart failure and control patients are much more separable after updating the encoder network using a classification loss. This allows for more targeted analysis of subgroups within the known heart failure patients whilst using representations from control patients to train an embedding model. This separation is quantified using classifiers, as described in the main paper, with the area under the receiver operating curve (AUROC) using DSEC being 0.84, while the AUROC is 0.73 using DEC and a random forest classifier, and 0.63 using PCA with a random forest classifier.

## 3. Hierarchical Clustering

The following sections aim to give a direct comparison between the three embedding methods: PCA (the baseline method), DEC (the state-of-the-art method), and DSEC (the novel extensions developed in this work). Clusters are compared through the mean and standard deviation of the blood measures and vital signs used to determine the embedded space, in addition to enrichment analysis performed between the pairs of clusters which are combined at each agglomeration step.

## 3.1. Principal Component Analysis

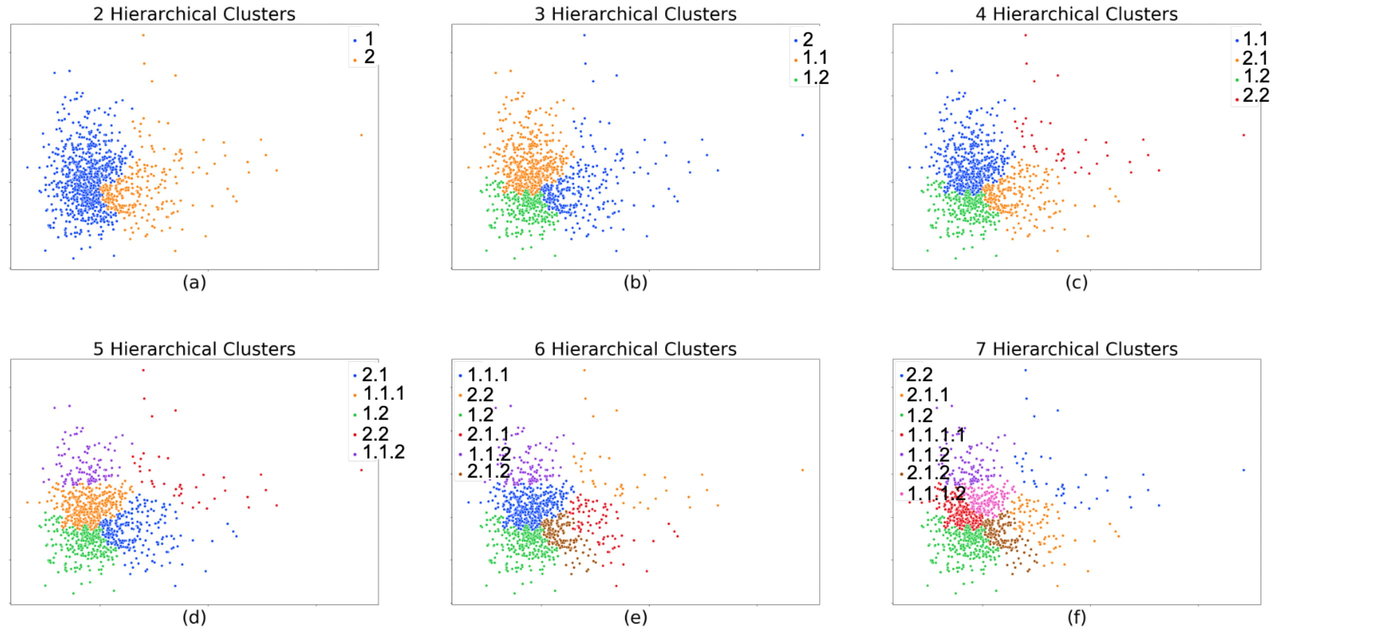


*Figure 3.* The embedded space found using PCA split from two to seven clustering using agglomerative clustering with the Ward criteria.

Figure 3 shows the first seven hierarchical clusters found using the PCA embeddings of the bloods measures and vital signs. The following tables describe the clusters using the average values of the features in each clusters and through enrichment of diagnoses which occur within clusters.

*Table 1.* Mean plus/minus standard deviation of the input features for the clusters found from Figure 3

| Cluster | 1 | 2 | 1.1 | 1.2 | 2.1 | 2.2 |
|---|---|---|---|---|---|---|
| Systolic BP | 134.7±19.92 | 124.2±18.01 | 128.5±15.73 | 145.3±21.87 | 125.7±17.58 | 115.0±18.17 |
| Diastolic BP | 72.14±10.10 | 65.16±8.602 | 69.76±8.954 | 76.28±10.65 | 65.69±8.378 | 61.80±9.336 |
| Heart Rate | 81.02±13.17 | 75.47±12.58 | 85.07±11.90 | 74.01±12.31 | 73.75±11.25 | 86.39±15.04 |
| Oxygen Sat. | 95.85±1.931 | 95.80±2.163 | 95.47±2.034 | 96.52±1.523 | 96.11±1.626 | 93.87±3.675 |
| Temperature | 36.41±0.348 | 36.19±0.328 | 36.50±0.326 | 36.26±0.337 | 36.19±0.315 | 36.23±0.404 |
| ALT | 27.86±42.50 | 40.80±81.82 | 31.68±51.88 | 21.23±14.29 | 36.43±73.96 | 68.49±117.7 |
| Creatinine | 85.14±28.67 | 176.0±108.6 | 83.82±28.90 | 87.42±28.16 | 158.5±86.39 | 286.5±160.4 |
| CRP | 45.34±54.32 | 44.08±64.10 | 63.43±60.21 | 13.93±15.16 | 28.17±26.55 | 144.7±119.0 |
| Platelets | 258.7±93.25 | 214.1±81.80 | 281.1±100.5 | 219.6±62.07 | 210.6±76.21 | 236.3±109.4 |
| Potassium | 3.974±0.427 | 4.536±0.654 | 3.963±0.432 | 3.993±0.420 | 4.472±0.581 | 4.944±0.912 |
| Sodium | 137.1±4.311 | 137.2±4.412 | 136.4±4.408 | 138.3±3.853 | 137.4±3.946 | 135.5±6.478 |
| Urea | 7.133±2.884 | 15.86±7.845 | 7.258±3.057 | 6.916±2.547 | 14.48±6.033 | 24.59±11.62 |
| White Cells | 9.583±3.648 | 8.631±3.822 | 10.79±3.798 | 7.486±2.111 | 7.900±2.522 | 13.25±6.551 |
| Cluster | 1.1.1 | 1.1.2 | 2.1.1 | 2.1.2 | 1.1.1.1 | 1.1.1.2 |
| Systolic BP | 129.1±15.18 | 126.4±17.42 | 124.9±18.40 | 126.1±17.22 | 133.9±14.34 | 122.3±13.73 |
| Diastolic BP | 70.18±8.900 | 68.28±9.029 | 64.81±9.854 | 66.11±7.580 | 73.37±7.984 | 65.53±8.100 |
| Heart Rate | 83.75±11.65 | 89.72±11.67 | 74.79±13.08 | 73.26±10.29 | 83.49±10.46 | 84.13±13.22 |
| Oxygen Sat. | 95.65±1.767 | 94.82±2.690 | 95.76±2.106 | 96.27±1.318 | 95.80±1.651 | 95.43±1.909 |
| Temperature | 36.44±0.277 | 36.69±0.406 | 36.21±0.330 | 36.18±0.308 | 36.44±0.260 | 36.44±0.301 |
| ALT | 32.02±55.70 | 30.49±35.38 | 49.10±117.1 | 30.46±39.10 | 25.30±23.11 | 41.79±81.88 |
| Creatinine | 83.92±28.36 | 83.47±30.89 | 225.1±112.1 | 127.2±45.03 | 74.22±20.90 | 98.04±31.72 |
| CRP | 46.37±45.47 | 123.7±67.02 | 39.05±29.56 | 23.04±23.40 | 34.24±34.60 | 64.01±53.10 |
| Platelets | 264.4±83.18 | 340.4±130.4 | 220.1±84.78 | 206.1±71.66 | 279.1±81.80 | 242.9±80.68 |
| Potassium | 3.983±0.420 | 3.891±0.464 | 4.698±0.591 | 4.365±0.546 | 3.871±0.366 | 4.146±0.441 |
| Sodium | 136.4±4.477 | 136.1±4.156 | 136.8±4.888 | 137.7±3.395 | 136.7±4.642 | 136.1±4.216 |
| Urea | 7.218±3.003 | 7.399±3.253 | 20.17±6.047 | 11.80±3.739 | 6.051±2.057 | 8.917±3.339 |
| White Cells | 9.856±2.858 | 14.09±4.766 | 8.580±2.517 | 7.579±2.467 | 9.466±2.565 | 10.42±3.160 |

Table 1 shows how the mean input features differ between the clusters found in Figure 3. For example cluster 2 is associated with high levels of creatinine and urea compared to cluster 1.

*Table 2.* Top five enriched ICD-10 codes between hierarchical splits in PCA clusters (log odds-ratio shown in brackets). Enrichment is performed between pairs of clusters, (for example 1 vs 2, 2.1 vs 2.2, and 1.1.1 vs 1.1.2).

| GROUP | ENRICHED ICD-10 CODES |
|---|---|
| 1 | |
| 2 | N18.9 CHRONIC RENAL FAILURE, UNSPECIFIED (1.82) |
| | I08.1 DISORDERS OF BOTH MITRAL AND TRICUSPID VALVES (1.09) |
| | N17.9 ACUTE RENAL FAILURE, UNSPECIFIED (1.57) |
| | Z95.0 PRESENCE OF CARDIAC PACEMAKER (0.99) |
| | I20.9 ANGINA PECTORIS, UNSPECIFIED (0.98) |
| 1.1 | J18.9 PNEUMONIA, UNSPECIFIED (2.08) |
| | J18.1 LOBAR PNEUMONIA, UNSPECIFIED (1.79) |
| | N17.9 ACUTE RENAL FAILURE, UNSPECIFIED (1.53) |
| | Z50.1 OTHER PHYSICAL THERAPY (1.35) |
| | N39.0 URINARY TRACT INFECTION, SITE NOT SPECIFIED (1.30) |
| 1.2 | |
| 2.1 | I50.0 CONGESTIVE HEART FAILURE (1.28) |
| 2.2 | Z51.5 PALLIATIVE CARE (2.93) |
| | E87.2 ACIDOSIS (2.68) |
| | J18.9 PNEUMONIA, UNSPECIFIED (1.91) |
| | N17.9 ACUTE RENAL FAILURE, UNSPECIFIED (1.43) |
| 1.1.1 | Z86.6 PERSONAL HISTORY OF DISEASES OF THE NERVOUS SYSTEM AND SENSE ORGANS (2.37) |
| 1.1.2 | Z51.5 PALLIATIVE CARE (1.70) |
| | A41.9 SEPTICAEMIA, UNSPECIFIED (1.69) |
| 2.1.1 | K57.3 DIVERTICULAR DISEASE OF LARGE INTESTINE WITHOUT PERFORATION OR ABSCESS (INF) |
| | E87.5 HYPERKALAEMIA (2.78) |
| | N17.9 ACUTE RENAL FAILURE, UNSPECIFIED (1.96) |
| | N18.9 CHRONIC RENAL FAILURE, UNSPECIFIED (1.18) |
| 2.1.2 | |
| 1.1.1.1 | |
| 1.1.1.2 | N17.9 ACUTE RENAL FAILURE, UNSPECIFIED (1.82) |
| | J18.1 LOBAR PNEUMONIA, UNSPECIFIED (1.43) |
| | J90 PLEURAL EFFUSION, NOT ELSEWHERE CLASSIFIED (0.83) |

Table 2 show the enriched ICD-10 codes found within the clusters defined in Figure 3. There are no clear splits between clusters associated with heart failure, with the exception of cluster 2.1 which in enriched with congestive heart failure diagnoses compared to cluster 2.2. It is difficult to draw any conclusions about subpopulations of heart failure patients with the lack of heart failure clusters.

## 3.2. Deep Embedded Clustering

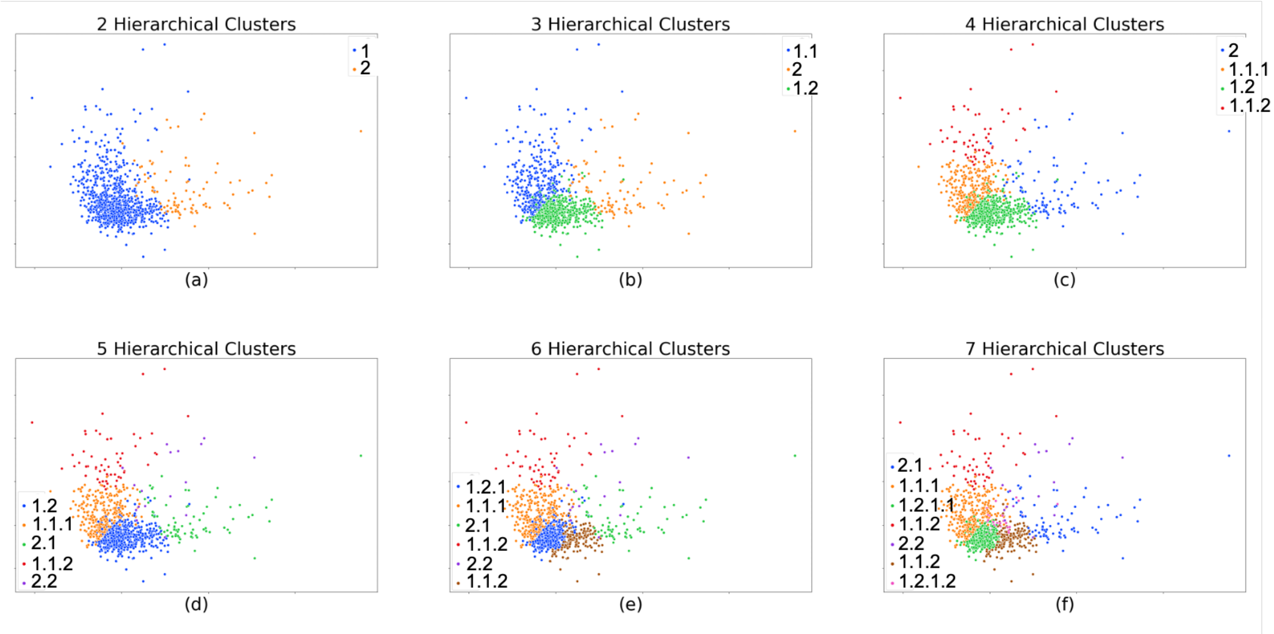


*Figure 4.* The embedded space found using DEC split from two to seven clustering using agglomerative clustering with the Ward criteria.

Figure 4 shows the first seven hierarchical clusters found using the DEC embeddings of the bloods measures and vital signs. The following tables describe the clusters using the average values of the features in each clusters and through enrichment of diagnoses which occur within clusters.

*Table 3.* Mean plus/minus standard deviation of the input features for the clusters found from Figure 4

| Cluster | 1 | 2 | 1.1 | 1.2 | 1.1.1 | 1.1.2 |
|---|---|---|---|---|---|---|
| Systolic BP | 132.6±19.85 | 124.3±19.74 | 132.0±16.71 | 133.0±21.36 | 131.9±16.97 | 132.4±15.36 |
| Diastolic BP | 70.66±10.18 | 66.46±9.653 | 69.43±8.862 | 71.33±10.78 | 69.49±9.040 | 69.14±7.934 |
| Heart Rate | 79.59±13.19 | 79.44±13.90 | 82.79±11.44 | 77.86±13.74 | 82.32±11.28 | 85.20±12.06 |
| Oxygen Sat. | 95.87±1.965 | 95.50±2.272 | 96.05±1.513 | 95.77±2.165 | 96.14±1.400 | 95.59±1.953 |
| Temperature | 36.36±0.356 | 36.25±0.345 | 36.49±0.353 | 36.30±0.340 | 36.44±0.334 | 36.70±0.378 |
| ALT | 25.70±22.85 | 93.26±167.8 | 27.73±26.61 | 24.60±20.48 | 27.96±27.65 | 26.56±20.54 |
| Creatinine | 94.68±37.17 | 267.8±146.9 | 83.02±29.55 | 100.9±39.30 | 81.16±25.99 | 92.74±42.70 |
| CRP | 43.57±57.37 | 61.13±50.28 | 80.75±78.66 | 23.51±24.21 | 55.70±47.01 | 211.5±81.40 |
| Platelets | 248.5±92.22 | 230.8±94.13 | 305.4±111.6 | 217.7±60.72 | 305.6±102.3 | 304.5±152.3 |
| Potassium | 4.064±0.493 | 4.759±0.768 | 4.022±0.462 | 4.087±0.508 | 4.024±0.437 | 4.009±0.581 |
| Sodium | 137.1±4.264 | 136.8±5.090 | 134.9±4.660 | 138.3±3.522 | 134.8±4.652 | 135.8±4.641 |
| Urea | 8.281±3.975 | 22.09±9.949 | 7.428±3.535 | 8.742±4.123 | 7.221±2.921 | 8.513±5.683 |
| White Cells | 9.218±3.501 | 10.63±5.445 | 11.32±4.020 | 8.082±2.547 | 10.75±3.373 | 14.29±5.579 |
| Cluster | 2.1 | 2.2 | 1.2.1 | 1.2.2 | 1.2.1.1 | 1.2.1.2 |
| Systolic BP | 124.8±19.53 | 122.0±21.10 | 134.8±20.84 | 127.1±22.08 | 135.0±20.99 | 132.2±19.10 |
| Diastolic BP | 66.03±9.186 | 68.36±11.62 | 72.96±10.80 | 65.93±8.785 | 73.28±10.73 | 69.37±11.02 |
| Heart Rate | 77.20±13.29 | 89.31±12.46 | 79.21±13.91 | 73.37±12.19 | 78.17±13.29 | 90.95±15.45 |
| Oxygen Sat. | 95.53±2.319 | 95.39±2.111 | 95.65±2.292 | 96.19±1.616 | 96.10±1.552 | 90.53±2.971 |
| Temperature | 36.23±0.344 | 36.32±0.350 | 36.36±0.305 | 36.11±0.377 | 36.35±0.292 | 36.38±0.429 |
| ALT | 29.27±45.86 | 375.6±215.9 | 24.93±21.33 | 23.52±17.37 | 24.88±21.51 | 25.46±19.42 |
| Creatinine | 297.9±142.7 | 135.0±74.97 | 88.56±27.80 | 142.0±43.69 | 87.72±26.33 | 98.09±40.00 |
| CRP | 65.77±53.13 | 40.63±27.81 | 22.29±22.48 | 27.58±28.94 | 20.97±21.28 | 37.04±29.71 |
| Platelets | 230.9±89.55 | 230.5±115.3 | 219.7±58.86 | 211.1±66.25 | 218.9±56.98 | 229.2±77.16 |
| Potassium | 4.806±0.659 | 4.550±1.133 | 3.976±0.416 | 4.454±0.606 | 3.959±0.386 | 4.171±0.639 |
| Sodium | 137.2±4.670 | 135.2±6.554 | 138.4±3.433 | 137.7±3.761 | 138.4±3.434 | 139.2±3.373 |
| Urea | 23.71±9.448 | 14.91±9.110 | 7.360±2.829 | 13.32±4.424 | 7.238±2.666 | 8.734±4.044 |
| White Cells | 10.14±4.334 | 12.77±8.704 | 8.049±2.443 | 8.189±2.870 | 7.982±2.370 | 8.805±3.085 |

Table 3 shows how the mean input features differ between the clusters found in Figure 4. For example cluster 2 is associated with high levels of creatinine and ALT compared to cluster 1.

*Table 4.* Top five enriched ICD-10 codes between hierarchical splits in DEC clusters (log odds-ratio shown in brackets). Enrichment is performed between pairs of clusters, (for example 1 vs 2, 2.1 vs 2.2, and 1.1.1 vs 1.1.2).

| Group | Enriched ICD-10 Codes |
|---|---|
| 1 | |
| 2 | Z99.2 Dependence on renal dialysis (inf) |
| | N18.5 Chronic kidney disease, stage 5 (4.58) |
| | E87.5 Hyperkalaemia (3.42) |
| | N18.4 Chronic kidney disease, stage 4 (1.96) |
| | I24.9 Acute ischaemic heart disease, unspecified (1.87) |
| 1.1 | E87.1 Hypo-osmolality and hyponatraemia (1.81) |
| | J18.9 Pneumonia, unspecified (1.11) |
| | Z50.1 Other physical therapy (0.85) |
| 1.2 | I20.9 Angina pectoris, unspecified (1.08) |
| | Z95.1 Presence of aortocoronary bypass graft (1.08) |
| | N18.9 Chronic renal failure, unspecified (1.03) |
| | I50.9 Heart failure, unspecified (0.79) |
| | I50.0 Congestive heart failure (0.79) |
| 1.1.1 | I50.0 Congestive heart failure (1.52) |
| 1.1.2 | G30.9 Alzheimer's disease, unspecified (3.10) |
| | F00.9 Dementia in Alzheimer's disease, unspecified (3.10) |
| | A41.5 Septicaemia due to other Gram-negative organisms (3.10) |
| | N17.9 Acute renal failure, unspecified (1.10) |
| 2.1 | |
| 2.2 | F32.9 Depressive episode, unspecified (2.57) |
| 1.2.1 | |
| 1.2.2 | N17.9 Acute renal failure, unspecified (1.74) |
| | N18.9 Chronic renal failure, unspecified (1.38) |
| | I51.7 Cardiomegaly (0.79) |
| | I50.0 Congestive heart failure (0.60) |
| 1.2.1.1 | |
| 1.2.1.2 | J96.91 Respiratory failure unspecified; Type II [hypercapnic] (3.90) |
| | Z86.1 Personal history of infectious and parasitic diseases (2.80) |
| | J44.0 Chronic obstructive pulmonary disease with acute lower respiratory infection (2.51) |
| | Z51.5 Palliative care (2.35) |
| | J44.9 Chronic obstructive pulmonary disease, unspecified (2.10) |

Table 4 show the enriched ICD-10 codes found within the clusters defined in Figure 4. There is no clear split between heart failure and control patients in clusters 1 and 2. Subsequent clusters are associated with heart failure, for example clusters 1.2, 1.1.1, and 1.2.2. However due to parent clusters not being associated with heart failure patients it is difficult to determine characteristics of subpopulations of heart failure. This can be seen in in cluster 1.2, as cluster 1 is not associated with heart failure, cluster 1.1 can not be linked to heart failure. Therefore cluster 1.2 may just contain patients with any form of heart failure rather than having a different type of heart failure compared to cluster 1.1.

### 3.3. Deep Semi-Supervised Embedded Clustering

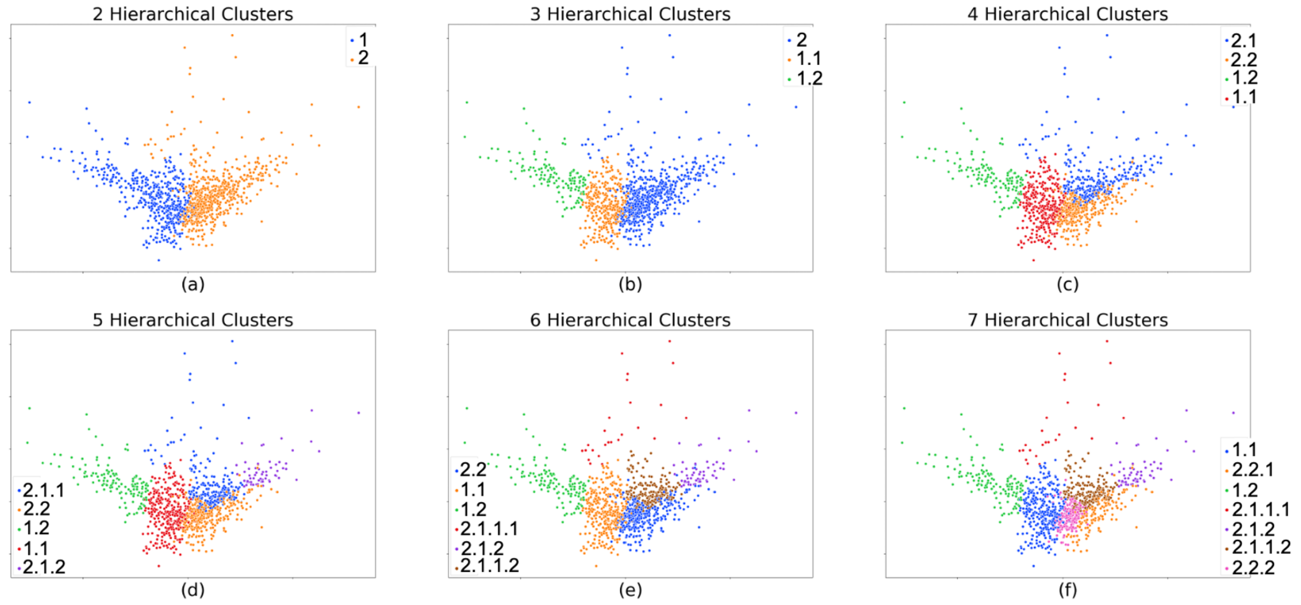


*Figure 5.* The embedded space found using DSEC split from two to seven clustering using agglomerative clustering with the Ward criteria.

Figure 5 shows the first seven hierarchical clusters found using the DSEC embeddings of the bloods measures and vital signs. The following tables describe the clusters using the average values of the features in each clusters and through enrichment of diagnoses which occur within clusters.

*Table 5.* Mean plus/minus standard deviation of the input features for the clusters found from Figure 5

| Cluster | 1 | 2 | 1.1 | 1.2 | 2.1 | 2.2 |
|---|---|---|---|---|---|---|
| Systolic BP | 136.5±19.86 | 128.5±19.37 | 138.8±21.00 | 130.6±15.14 | 122.3±16.88 | 133.6±19.80 |
| Diastolic BP | 70.00±9.766 | 70.56±10.52 | 71.30±9.819 | 66.66±8.821 | 66.06±8.169 | 74.23±10.80 |
| Heart Rate | 78.08±12.63 | 80.70±13.58 | 76.77±12.50 | 81.44±12.39 | 76.30±11.96 | 84.29±13.79 |
| Oxygen Sat. | 96.45±1.667 | 95.38±2.095 | 96.51±1.647 | 96.28±1.712 | 96.16±1.433 | 94.75±2.324 |
| Temperature | 36.49±0.390 | 36.26±0.293 | 36.41±0.369 | 36.67±0.381 | 36.19±0.299 | 36.31±0.277 |
| ALT | 24.50±21.37 | 36.30±71.03 | 24.15±21.97 | 25.38±19.82 | 50.65±101.4 | 24.59±21.90 |
| Creatinine | 85.88±41.01 | 126.1±85.38 | 87.08±43.86 | 82.80±32.51 | 159.7±104.9 | 98.73±51.06 |
| CRP | 69.36±72.98 | 26.73±30.29 | 40.32±37.80 | 143.8±87.43 | 32.13±37.14 | 22.34±22.38 |
| Platelets | 259.1±97.69 | 237.9±87.32 | 250.7±86.22 | 280.7±119.9 | 215.6±77.37 | 256.2±90.77 |
| Potassium | 4.024±0.468 | 4.194±0.602 | 4.044±0.453 | 3.972±0.502 | 4.413±0.651 | 4.015±0.491 |
| Sodium | 136.7±3.997 | 137.4±4.556 | 137.0±3.984 | 136.0±3.961 | 136.0±4.808 | 138.5±4.028 |
| Urea | 7.080±3.437 | 11.16±6.973 | 7.094±3.148 | 7.047±4.099 | 14.61±8.158 | 8.354±4.062 |
| White Cells | 10.50±3.905 | 8.457±3.310 | 9.611±3.386 | 12.78±4.218 | 8.743±4.092 | 8.224±2.480 |
| Cluster | 2.1.1 | 2.1.2 | 2.1.1.1 | 2.1.1.2 | 2.2.1 | 2.2.2 |
| Systolic BP | 124.4±16.01 | 114.6±17.91 | 122.0±19.34 | 124.7±15.56 | 129.2±20.51 | 136.7±18.71 |
| Diastolic BP | 66.86±7.763 | 63.10±8.991 | 66.02±10.29 | 66.97±7.400 | 74.85±12.57 | 73.80±9.371 |
| Heart Rate | 77.32±11.64 | 72.49±12.46 | 85.07±10.94 | 76.32±11.37 | 88.16±15.67 | 81.55±11.56 |
| Oxygen Sat. | 96.14±1.307 | 96.23±1.836 | 95.51±1.967 | 96.22±1.179 | 93.84±2.883 | 95.39±1.545 |
| Temperature | 36.21±0.277 | 36.10±0.357 | 36.33±0.358 | 36.20±0.262 | 36.25±0.286 | 36.35±0.264 |
| ALT | 54.29±110.0 | 37.11±57.65 | 212.0±258.3 | 33.89±41.20 | 27.30±28.69 | 22.68±15.21 |
| Creatinine | 152.2±109.8 | 187.6±78.84 | 255.2±191.0 | 138.8±86.62 | 113.8±62.26 | 88.07±38.08 |
| CRP | 34.99±40.17 | 21.47±19.32 | 96.36±64.86 | 27.05±27.28 | 22.56±19.77 | 22.18±24.09 |
| Platelets | 222.7±76.71 | 189.2±74.64 | 225.6±113.4 | 222.3±70.98 | 241.7±85.97 | 266.4±92.85 |
| Potassium | 4.371±0.628 | 4.570±0.712 | 4.676±1.060 | 4.332±0.540 | 4.026±0.535 | 4.007±0.459 |
| Sodium | 136.4±4.524 | 134.6±5.568 | 136.4±4.922 | 136.4±4.483 | 138.7±3.803 | 138.3±4.182 |
| Urea | 13.06±7.619 | 20.34±7.566 | 22.06±14.40 | 11.90±5.267 | 9.974±4.921 | 7.211±2.823 |
| White Cells | 9.207±4.325 | 7.015±2.401 | 15.50±8.379 | 8.393±2.559 | 7.666±2.393 | 8.617±2.470 |

Table 5 shows how the mean input features differ between the clusters found in Figure 5. For example cluster 1 is associated with high levels of CRP and low levels of creatinine compared to cluster 2.

*Table 6.* Top five enriched ICD-10 codes between hierarchical splits in DSEC clusters (log odds-ratio shown in brackets). Enrichment is performed between pairs of clusters, (for example 1 vs 2, 2.1 vs 2.2, and 1.1.1 vs 1.1.2).

| Group | Enriched ICD-10 Codes |
|---|---|
| 1 | E78.0 Pure hypercholesterolaemia (0.96) |
| 2 | I50.0 Congestive heart failure (1.69) |
| | E87.7 Fluid overload (1.39) |
| | I50.9 Heart failure, unspecified (1.32) |
| | N18.9 Chronic renal failure, unspecified (1.22) |
| | I34.0 Mitral (valve) insufficiency (1.17) |
| 1.1 | I25.9 Chronic ischaemic heart disease, unspecified (1.56) |
| 1.2 | |
| 2.1 | I42.0 Dilated cardiomyopathy (1.56) |
| | N17.9 Acute renal failure, unspecified (1.37) |
| | N39.0 Urinary tract infection, site not specified (1.34) |
| | N18.9 Chronic renal failure, unspecified (1.04) |
| | Z95.1 Presence of aortocoronary bypass graft (1.10) |
| 2.2 | |
| 2.1.1 | I50.1 Left ventricular failure (2.35) |
| 2.1.2 | R18 Ascites (3.00) |
| | E87.5 Hyperkalaemia (2.13) |
| | I42.0 Dilated cardiomyopathy (1.55) |
| | I50.0 Congestive heart failure (1.16) |
| | N17.9 Acute renal failure, unspecified (1.15) |
| 2.1.1.1 | E87.5 Hyperkalaemia (3.26) |
| | Z51.5 Palliative care (2.69) |
| 2.1.1.2 | |
| 2.2.1 | I27.2 Other secondary pulmonary hypertension (2.91) |
| | N18.9 Chronic renal failure, unspecified (1.45) |
| | I48.9 Atrial fibrillation and atrial flutter, unspecified (1.36) |
| | E87.7 Fluid overload (1.09) |
| | Z92.1 Personal history of long-term (current) use of anticoagulants (0.95) |
| 2.2.2 | |

Table 6 show the enriched ICD-10 codes found within the clusters defined in Figure 5. The first split between clusters 1 and 2 clearly shows cluster 2 is associated with heart failure diagnoses, whereas cluster 1 is not. Cluster 2 is then split into a cluster 2.1 which is heart failure associated with cardiomyopathy, renal failure, and aortocoronary bypass grafts. Cluster 2.1 can be further split in to cluster 2.1.1, associated with left ventricular failure, and cluster 2.1.2, associated with ascites and hyperkalaemia. Cluster 2.2 can also be further split in to cluster 2.2.1, associated with pulmonary hypertension, atrial fibrillation and flutter, fluid overload, and use of anticoagulants.

The ability to first split known cohorts using a classification task allows for a much more interpretable method of determining subgroups within the cohort of interest. This can be seen through the labels shown in Figure 2, in addition to the enriched diagnoses codes in Tables 2, 4, and 6, through use of only commonly recorded blood measures and vital signs.
